# Supplementary material for: Horizon physics of quasi-one-dimensional tilted Weyl cones on a lattice
Source: arXiv:2206.04138 ancillary file (2022-06-08)
Supplement: Supplementary file 1 [file supplemental.pdf]

# Supplemental Material - Horizon physics of quasi-one-dimensional tilted Weyl cones on a lattice

Viktor Könye,<sup>1</sup> Corentin Morice,<sup>2,3</sup> Dmitry Chernyavsky,<sup>1</sup> Ali G. Moghaddam,<sup>4,5</sup> Jeroen van den Brink,<sup>1,6</sup> and Jasper van Wezel<sup>2</sup>

<sup>1</sup>*Institute for Theoretical Solid State Physics, IFW Dresden and Würzburg-Dresden Cluster of Excellence ct.qmat, Helmholtzstr. 20, 01069 Dresden, Germany*

<sup>2</sup>*Institute for Theoretical Physics and Delta Institute for Theoretical Physics, University of Amsterdam, 1090 GL Amsterdam, The Netherlands*

<sup>3</sup>*Laboratoire de Physique des Solides, CNRS UMR 8502, Université Paris-Saclay, F-91405 Orsay Cedex, France*

<sup>4</sup>*Department of Physics, Institute for Advanced Studies in Basic Sciences (IASBS), Zanjan 45137-66731, Iran*

<sup>5</sup>*Computational Physics Laboratory, Physics Unit, Faculty of Engineering and Natural Sciences, Tampere University, FI-33014 Tampere, Finland*

<sup>6</sup>*Institute for Theoretical Physics, TU Dresden, 01069 Dresden, Germany*

(Dated: June 6, 2022)

In this supplemental material we list the file names and parameters of all animations corresponding to the figures in the main paper.

## I. 1D RESULTS

The animations for Fig. 4 are listed in Tab. I. Here the linear tilting dependence was used

$$t(x) = 2x/L. \quad (1)$$

| File name      | $H$        | $L$  | $x_0$ | $\sigma$ | $k$  |
|----------------|------------|------|-------|----------|------|
| 1d_H1_k0.mp4   | $H_1^{1D}$ | 1000 | 100   | 50       | 0.00 |
| 1d_H1_k005.mp4 | $H_1^{1D}$ | 1000 | 100   | 50       | 0.05 |
| 1d_H1_k01.mp4  | $H_1^{1D}$ | 1000 | 100   | 50       | 0.10 |
| 1d_H1_k015.mp4 | $H_1^{1D}$ | 1000 | 100   | 50       | 0.15 |
| 1d_H2_k0.mp4   | $H_2^{1D}$ | 1000 | 100   | 50       | 0.00 |
| 1d_H2_k005.mp4 | $H_2^{1D}$ | 1000 | 100   | 50       | 0.05 |
| 1d_H2_k01.mp4  | $H_2^{1D}$ | 1000 | 100   | 50       | 0.10 |
| 1d_H2_k015.mp4 | $H_2^{1D}$ | 1000 | 100   | 50       | 0.15 |

Table I. Animations for Fig. 4 of the main paper. The position dependence of the tilting is Eq. (1).  $H$  is the Hamiltonian,  $L$  is the length of the system,  $x_0$  is the initial position of the wave packet,  $\sigma$  is the width of the wave packet, and  $k$  is the initial momentum.

The animations for Fig. 9 panels (a) and (b) are listed in Tab. II. Here the position dependence of the tilting follows a power law with exponent  $\gamma$

$$t(x) = 1 + \text{sgn}(2x - L) \left| \frac{2x}{L} - 1 \right|^\gamma. \quad (2)$$

The animations for Fig. 9 panels (c) and (d) are listed in Tab. III. The position dependence of the tilting is

$$t(x) = 1 - \sqrt{\left(\frac{2x}{L} - 1\right)^2 + \left(\frac{2x_0}{L} - 1\right)^2} \tan^2 k. \quad (3)$$

| File name             | $H$        | $L$  | $\gamma$ | $x_0$ | $\sigma$ | $k$ |
|-----------------------|------------|------|----------|-------|----------|-----|
| 1d_power05_H1_k0.mp4  | $H_1^{1D}$ | 1000 | 0.5      | 100   | 50       | 0.0 |
| 1d_power1_H1_k0.mp4   | $H_1^{1D}$ | 1000 | 1.0      | 100   | 50       | 0.0 |
| 1d_power2_H1_k0.mp4   | $H_1^{1D}$ | 1000 | 2.0      | 100   | 50       | 0.0 |
| 1d_power05_H1_k01.mp4 | $H_1^{1D}$ | 1000 | 0.5      | 100   | 50       | 0.1 |
| 1d_power1_H1_k01.mp4  | $H_1^{1D}$ | 1000 | 1.0      | 100   | 50       | 0.1 |
| 1d_power2_H1_k01.mp4  | $H_1^{1D}$ | 1000 | 2.0      | 100   | 50       | 0.1 |

Table II. Animations for Fig. 9 panels (a) and (b) of the main paper. The position dependence of the tilting is Eq. (2).  $\gamma$  is the exponent. The rest of the symbols are as in Tab. I.

| File name                | $H$        | $L$  | $x_0$ | $\sigma$ | $k$ |
|--------------------------|------------|------|-------|----------|-----|
| 1d_H1_k0.mp4             | $H_1^{1D}$ | 1000 | 100   | 50       | 0.0 |
| 1d_H1_k02.mp4            | $H_1^{1D}$ | 1000 | 100   | 50       | 0.2 |
| 1d_artificial_H1_k02.mp4 | $H_1^{1D}$ | 1000 | 100   | 50       | 0.2 |
| 1d_H1_k05.mp4            | $H_1^{1D}$ | 1000 | 100   | 50       | 0.5 |
| 1d_artificial_H1_k05.mp4 | $H_1^{1D}$ | 1000 | 100   | 50       | 0.5 |

Table III. Animations for Fig. 9 panels (c) and (d) of the main paper. The position dependence of the tilting for the file names that contain artificial is Eq. (3) for the rest it is Eq. (1). The symbols are as in Tab. I.

## II. 2D RESULTS

The animations for Fig. 6 are listed in Tab. IV. Here the tilting parameter is zero.

| File name            | $H$        | $L$ | $W$ | $x_0$ | $y_0$ | $\sigma$ | $k$ |
|----------------------|------------|-----|-----|-------|-------|----------|-----|
| 2d_H1_notilt_k0.mp4  | $H_1^{2D}$ | 500 | 500 | 250   | 250   | 20       | 0.0 |
| 2d_H1_notilt_k01.mp4 | $H_1^{2D}$ | 500 | 500 | 250   | 250   | 20       | 0.1 |
| 2d_H1_notilt_k02.mp4 | $H_1^{2D}$ | 500 | 500 | 250   | 250   | 20       | 0.2 |

Table IV. Animations for Fig. 6 of the main paper. The tilting is zero everywhere.  $W$  is the width of the system and  $y_0$  is the initial  $y$  coordinate of the wave packet. The rest of the symbols are as in Tab. I.

The animations for Fig. 7 are listed in Tab. V. Here the linear tilting dependence was used as in Eq. (1).

## III. 3D RESULTS

The animations for Fig. 8 are listed in Tab. VI. Here the linear tilting dependence was used similar to Eq. (1)

$$t(x) = x/L. \quad (4)$$

| File name      | $H$        | $L$ | $W$ | $x_0$ | $y_0$ | $\sigma$ | $k$  |
|----------------|------------|-----|-----|-------|-------|----------|------|
| 2d_H1_k0.mp4   | $H_1^{2D}$ | 500 | 500 | 100   | 250   | 40       | 0.00 |
| 2d_H1_k005.mp4 | $H_1^{2D}$ | 500 | 500 | 100   | 250   | 40       | 0.05 |
| 2d_H1_k01.mp4  | $H_1^{2D}$ | 500 | 500 | 100   | 250   | 40       | 0.10 |
| 2d_H1_k015.mp4 | $H_1^{2D}$ | 500 | 500 | 100   | 250   | 40       | 0.15 |
| 2d_H2_k0.mp4   | $H_2^{2D}$ | 500 | 500 | 100   | 250   | 40       | 0.00 |
| 2d_H2_k005.mp4 | $H_2^{2D}$ | 500 | 500 | 100   | 250   | 40       | 0.05 |
| 2d_H2_k01.mp4  | $H_2^{2D}$ | 500 | 500 | 100   | 250   | 40       | 0.10 |
| 2d_H2_k015.mp4 | $H_2^{2D}$ | 500 | 500 | 100   | 250   | 40       | 0.15 |

Table V. Animations for Fig. 7 of the main paper. The position dependence of the tilting is Eq. (1). The symbols are as in Tab. IV.

| File name      | $H$        | $L$ | $W$ | $H$ | $x_0$ | $y_0$ | $z_0$ | $\sigma$ | $k$  |
|----------------|------------|-----|-----|-----|-------|-------|-------|----------|------|
| 3d_H1_k0.mp4   | $H_1^{3D}$ | 200 | 300 | 300 | 50    | 150   | 150   | 30       | 0.00 |
| 3d_H1_k005.mp4 | $H_1^{3D}$ | 200 | 300 | 300 | 50    | 150   | 150   | 30       | 0.05 |
| 3d_H1_k01.mp4  | $H_1^{3D}$ | 200 | 300 | 300 | 50    | 150   | 150   | 30       | 0.10 |
| 3d_H1_k015.mp4 | $H_1^{3D}$ | 200 | 300 | 300 | 50    | 150   | 150   | 30       | 0.15 |

Table VI. Animations for Fig. 8 of the main paper. The position dependence of the tilting is Eq. (4).  $H$  is the height of the system and  $z_0$  is the initial  $z$  coordinate of the wave packet. The rest of the symbols are as in Tab. IV.
